# Supplementary material for: ZTaint-Havoc: From Havoc Mode to Zero-Execution Fuzzing-Driven Taint Inference
Source: arXiv:2506.08838 source file (2025-06-10)
Supplement: Supplementary file 1 [file appendix.tex]

\section{Performance Characteristics}
\subsection{Mann-Whitney U Test \label{eval:mann-whitney-u}}
\begin{table}[!h]
\caption{\small\textbf{Mann-Whitney U test results of \sys against \aflpp, \sysdict against \aflppdict on \numfuzzbench FuzzBench programs for 24 hours over 10 runs. Statistically significant results ($p < 0.05$) are in bold.}}
    \label{eval:fuzzbench_sign}
    \begin{tabular}{lrr}
        \toprule
        \textbf {Targets} & \textbf{\aflpp} &\textbf{\aflppdict} \\ 
        \midrule
    bloaty & 2.41e-01 \\
    curl & 4.73e-01 \\
    libxslt & 8.20e-01 \\
    harfbuzz & 3.45e-01 \\
    jsoncpp & 7.26e-01 \\
    lcms & 1.21e-01 \\
    libjpeg & 7.72e-01 \\
    libpcap & 1.67e-01 \\
    libpng\_read\_fuzzer & \textbf{3.93e-02} \\
    libxml2\_xml & 9.70e-01 \\
    vorbis & 9.70e-01 \\
    openh264 & 9.10e-01 \\
    openssl & 2.10e-01 \\
    woff2 & 9.62e-02 \\
    zlib & 6.92e-01 \\
    re2 & 2.26e-01 \\
    sqlite3 & 1.62e-01 \\
    stbi & 8.21e-01 \\
    systemd & 3.40e-01 \\
        \bottomrule
    \end{tabular}
\end{table}

\begin{table}[!h]
\caption{\small\textbf{Mann-Whitney U test results of \sys against \aflpp, and \sysdict against \aflppdict, on \numstandalone standalone programs for 24 hours over 10 runs. Statistically significant results ($p < 0.05$) are in bold.}}
    \label{eval:standalone_sign}
    \begin{tabular}{lrr}
        \toprule
        \textbf {Targets} & \textbf{\aflpp} & \textbf{\aflppdict} \\ 
        \midrule
    exiv2     & 3.45e-01 \\
    tiffsplit & 4.73e-01 \\
    mp3gain   & 1.49e-01 \\
    mujs      & 4.73e-01 \\
    pdftotext & 4.73e-01 \\
    infotocap & 3.64e-01 \\
    mp42aac   & \textbf{4.59e-03} \\
    flvmeta   & \textbf{3.86e-02} \\
    objdump   & \textbf{2.33e-02} \\
    tcpdump   & \textbf{1.83e-04} \\
    ffmpeg    & 1.40e-01 \\
    jq        & 9.57e-02 \\
    cflow     & 4.26e-01 \\
    nm-new    & \textbf{5.80e-03} \\
    sqlite3   & \textbf{1.83e-04} \\
    lame      & 8.79e-01 \\
    jhead     & 1.00e+00 \\
        \bottomrule
    \end{tabular} 
\end{table}

\subsection{Coverage-over-time\label{app:coverage}}
